# Supplementary material for: ZeroSumEval: An Extensible Framework For Scaling LLM Evaluation with Inter-Model Competition
Source: arXiv:2503.10673 source file (2025-04-17)
Supplement: Supplementary file 1 [file 90_appendix.tex]

% \input{tables/model_versions}
% TODO: this figure looks very weird in this template. @Haidar any easy way to fix this?
% \begin{wrapfigure}[24]{R}{0.5\linewidth}
% \vspace{-1em}
%     \begin{center}
%     \begin{tikzpicture}[
%         box/.style={rectangle, draw, rounded corners, fill=blue!10, drop shadow, minimum height=0.8cm, minimum width=2.8cm, align=center},
%         boxllm/.style={rectangle, draw, rounded corners, fill=green!10, drop shadow, minimum height=0.8cm, minimum width=2.8cm, align=center},
%         actor/.style={circle, fill=white!10, draw, drop shadow, minimum size=0.8cm},
%         arrow/.style={-Stealth, thick, draw=black!80},
%         node distance=1cm and 2cm
%     ]

%     % Actors
%     \node[actor, label=above:{\textbf{Manager}}] (manager) at (-2, 0.5) {M};
%     \node[actor, label=above:{\textbf{Generator}}] (generator) at (2, 0.5) {G};

%     % Nodes for Manager
%     \node[box, below=of manager] (generate) {Generate Target};
%     \node[box, below=of generate] (verify) {Verification};
%     \node[box, below=of verify] (match) {Match Target?};

%     % Nodes for Generator
%     \node[boxllm, below=of generator] (genModel) {Receive Target};
%     \node[boxllm, below=of genModel] (output) {Generate Challenge};
%     \node[boxllm, below=of output] (clear) {Solve Challenge};

%     % Arrows between Manager and Generator
%     \draw[arrow] (generate) -- (genModel) node[midway, above, font=\small] {Target};
%     \draw[arrow] (genModel) -- (output);
%     \draw[arrow] (output) -- (verify);
%     \draw[arrow] (verify) -- (clear) node[midway, above, sloped, font=\small] {Clear};
%     \draw[arrow] (clear) -- (match);

%     % Dashed line separating roles
%     \draw[dashed, thick, dash pattern=on 5pt off 10pt] (0, 1) -- (0, -5.5) node[midway, right, fill=white, inner sep=1pt] {};


%     % Labels for clarity
%     \node[above=0.2cm of manager] (manager_label) {};
%     \node[above=0.2cm of generator] (generator_label) {};

%     \end{tikzpicture}
%     \end{center}
%     \caption{State diagram of the verification process involving the Game Manager and the Generator. Blue boxes indicate deterministic steps and green boxes indicate steps involving the model.}
%     \label{fig:state-diagram-verification}
% \end{wrapfigure}
% \input{tables/games}
